# Supplementary material for: Grassmann: The Coordinate-Independent Linear Algebra Programming Language
Source: arXiv:2611.00182 source file (2026-10-30)
Supplement: Supplementary file 1 [file helpers.tex]

\makeatletter
\newcommand{\gljudghead}[1]{\gl@get{judg@head}{#1}}
\newcommand{\gljudgdesc}[1]{\gl@get{judg@desc}{#1}}
\makeatother
\newcommand{\gldefnblock}[1]{\par\smallskip\noindent\textbf{\gldefnname{#1}}\par\nopagebreak\gldefn{#1}}
\newcommand{\appgrammar}[2]{\subsection{#2}\label{app:gen-syntax:#1}\begin{center}{\scriptsize\begin{tabular}{rclp{4.6cm}}\glsyntaxtable{#1}\end{tabular}}\end{center}}

%
%
%
\glsetnamepos{above}
\makeatletter
\renewcommand{\glrule}[2][]{\begingroup
  \def\gl@layout{#1}%
  \ifx\gl@layout\@empty
    \inferrule*[lab=\glrulename{#2}]
      {{\gl@premarray{#2}}}{{\gl@conclarray{#2}}}%
  \else
    \gl@premcollect{#2}\gl@prbuild{#1}%
    \ifnum\value{gl@premi}<\value{gl@premc}
      \PackageError{glang-lean}{Premise layout for #2 omits premises}
        {Supply enough premise slots in the optional argument.}%
    \fi
    \inferrule*[lab=\glrulename{#2}]
      {{\begin{array}{@{}c@{}}\gl@prows\end{array}}}
      {{\gl@conclarray{#2}}}%
  \fi\endgroup}
\makeatother
\let\glrules\glrulesnamed

%
%
%
\makeatletter
\def\gl@splitcob#1\xlongleftrightarrow#2#3\gl@stop{%
  \def\gl@shortconclusion{#1\xlongleftrightarrow{\leev_{\mathrm{out}}}#3}%
  \def\gl@outputprogram{#2}}
\newcommand{\glcobrule}[1]{%
  \begingroup\small
  \expandafter\let\expandafter\gl@rawconclusion\csname gl@rule@concl@#1\endcsname
  \expandafter\gl@splitcob\gl@rawconclusion\gl@stop
  \renewcommand{\glruleconcl}[1]{\gl@shortconclusion}%
  \glrulev{#1}%
  \par\medskip\noindent where
  \renewcommand{\LTTT}[3]{\textcolor{lang}{\MTM{}_{##1}}%
    \left\langle\begin{gathered}##2,\\[3pt]##3\end{gathered}\right\rangle}%
  \[\gpfit{\leev_{\mathrm{out}}=\gl@outputprogram}\]
  \endgroup}
\newcommand{\glcobrulepage}[1]{\clearpage\glcobrule{#1}\clearpage}

%
%
\def\gl@splitordinaryterm\evalJudge#1#2#3#4\gl@stop{%
  \def\gl@shortconclusion{\evalJudge{#1}{#2}{#3}{\leev_{\mathrm{out}}}}%
  \def\gl@outputprogram{#4}}
\def\gl@splitcheckedterm#1\xlongrightarrow#2#3\glresulttype#4\gl@stop{%
  \def\gl@shortconclusion{#1\xlongrightarrow{#2}\leev_{\mathrm{out}}\glresulttype{#4}}%
  \def\gl@outputprogram{#3}}
\newcommand{\gltermrule}[2][ordinary]{%
  \begingroup\small
  \expandafter\let\expandafter\gl@rawconclusion\csname gl@rule@concl@#2\endcsname
  \ifstrequal{#1}{checked}
    {\expandafter\gl@splitcheckedterm\gl@rawconclusion\gl@stop}
    {\expandafter\gl@splitordinaryterm\gl@rawconclusion\gl@stop}%
  \renewcommand{\glruleconcl}[1]{\gl@shortconclusion}%
  \glrulev{#2}%
  \par\nopagebreak\noindent where
  \[\gpfit{\leev_{\mathrm{out}}=\gl@outputprogram}\]
  \endgroup}
\makeatother

%
\makeatletter
\newcommand{\appstatementinput}[1]{\begingroup
  \emergencystretch=2em
  \let\label\@gobble\let\ltx@label\@gobble
  \input{tex/statements/#1}\par\endgroup}
\makeatother

%
%
%
\newcommand{\appRuleExplanation}[1]{%
  \par\nopagebreak[4]\smallskip\nopagebreak[4]
  \noindent\glruleexplanation{#1}\par}
\newcommand{\appRule}[1]{%
  \begin{samepage}\glrulev{#1}\appRuleExplanation{#1}\end{samepage}\medskip}
\newcommand{\appTermRule}[1]{%
  \begin{samepage}\gltermrule{#1}\appRuleExplanation{#1}\end{samepage}\medskip}
